# Supplementary material for: Failed Reasoning Traces Tell You What Is Fixable (But Not by Reading Them)
Source: arXiv:2606.05145 source file (2026-06-03)
Supplement: Supplementary file 1 [file emnlp_appendix_qualitative.tex]

% emnlp_appendix_qualitative.tex
% Auto-curated examples from routing_hierarchical_final.parquet.
% Requires: tcolorbox (with skins), booktabs, pifont, xcolor (added to preamble).

\providecommand{\cmark}{\textcolor{green!55!black}{\ding{51}}}
\providecommand{\xmark}{\textcolor{red!65!black}{\ding{55}}}

%% -----------------------------------------------------------------------
%  Feature glossary
%% -----------------------------------------------------------------------
\begin{tcolorbox}[breakable, width=\columnwidth,
  
  title={\textbf{Geometric feature glossary}},
  colback=blue!3, colframe=blue!40!black,
  fonttitle=\small\bfseries, before skip=4pt, after skip=8pt,
  left=4pt, right=4pt, top=3pt, bottom=3pt]
{\small
\begin{description}[leftmargin=1.8em, labelindent=0pt, itemsep=1pt, parsep=0pt]
  \item[$\Delta_{\mathrm{frac+}}$] Fraction of trajectory positions where the specialist is
    demonstrably worse than the ancestor (positive demotion). Low\,($<$0.1)\,=\,\emph{punctate};
    high\,($>$0.4)\,=\,\emph{distributed} across the full sequence.
  \item[feat\_conc] $J_{\max}/J_{\text{mean}}$: peakedness of the junction signal.  High means
    deformation is concentrated at one spike; low means no single injection point dominates.
  \item[spike pos.] Relative position of the largest junction spike in the token
    sequence ($t^*/L$). Identifies \emph{where} in the reasoning the concentrated deformation occurs.
  \item[$G_{\mathrm{cov,frac+}}$] Fraction of steps where the ancestor spans probability mass
    the specialist has lost. High values indicate structurally hard-to-repair, diffuse forgetting.
\end{description}
}
\end{tcolorbox}

%% -----------------------------------------------------------------------
%  Example 1 — Punctate spike, late in trace, SL-G rescues
%% -----------------------------------------------------------------------
\begin{tcolorbox}[breakable, width=\columnwidth,
  
  title={%
    \textbf{Ex.\,1:\ Punctate late spike — SL-G rescues}
    \hfill{\small\texttt{sft-1.7B}, CruxEval \texttt{sample\_469}, $k=1$}},
  colback=green!3, colframe=green!40!black,
  fonttitle=\small\bfseries, before skip=6pt, after skip=4pt,
  left=4pt, right=4pt, top=3pt, bottom=3pt]
{\small
\textbf{Task.}  Predict the output of a string-insertion function with modular-index logic.
\textbf{Call:} \texttt{f('sduyai',\,1,\,'y')} \quad \textbf{Expected:} \texttt{'syduyi'}

\medskip
\textbf{Failed rollout.}
\begin{quote}\ttfamily\footnotesize
\textlangle think\textrangle\textlangle/think\textrangle\enspace sduyay
\end{quote}
The model collapses reasoning and guesses one character off.

\medskip
\textbf{Junction spike:} token \textbf{786 / 1024} (\textbf{77\%} through the trace) —
at the final string-assembly step, where the one-character error is introduced.

\medskip
\textbf{Interpretation.}
The deformation is \emph{punctate} ($\Delta_{\mathrm{frac+}}{=}0.045$): nearly the entire trace
is intact, and the failure is mechanistically isolated to a single late-stage assembly step.
Junction concentration (feat\_conc\,=\,432) confirms one spike dominates at $432\times$ the mean.
A single logit injection at token 786 restores the correct output; retry ($T{=}0.6$) cannot
locate a silent, late spike by chance.

\medskip
\textbf{Repair:} retry=\xmark\enspace SL-G=\cmark\enspace DL=\cmark\enspace temp=\cmark\enspace temp\_loc=\cmark
}
\end{tcolorbox}

%% -----------------------------------------------------------------------
%  Example 2 — Punctate spike, detector missed it
%% -----------------------------------------------------------------------
\begin{tcolorbox}[breakable, width=\columnwidth,
  
  title={%
    \textbf{Ex.\,2:\ Punctate spike, detector missed — SL-G would rescue}
    \hfill{\small\texttt{sft-1.7B}, CruxEval \texttt{sample\_683}, $k=1$}},
  colback=orange!4, colframe=orange!50!black,
  fonttitle=\small\bfseries, before skip=6pt, after skip=4pt,
  left=4pt, right=4pt, top=3pt, bottom=3pt]
{\small
\textbf{Task.}  Predict the output of a dict-merge function.\\
\textbf{Call:} \texttt{f(\{'disface':9,'cam':7\},\,\{'mforce':5\})} \quad
\textbf{Expected:} \texttt{\{'disface':9,'cam':7,'mforce':5\}}

\medskip
\textbf{Failed rollout.}
\begin{quote}\ttfamily\footnotesize
\textlangle think\textrangle\textlangle/think\textrangle\enspace
The output of f(\ldots) is `\{'disface': 9, 'cam': 7, 'mforce': 5\}'.
\end{quote}
Correct-looking answer, wrong output format — string-match failure.

\medskip
\textbf{Junction spike:} detector fired at an uninformative step ($J_{\hat{t}}{=}0$);
the real spike exists elsewhere but was not located.

\medskip
\textbf{Interpretation.}
The deformation is again \emph{punctate} ($\Delta_{\mathrm{frac+}}{=}0.050$): a single bad step
exists and SL-G would rescue it.
The failure here is in \emph{detector precision}: peak ratio\,=\,0 means the injection
targeted a step where the ancestor--specialist gap is zero, leaving the actual spike
unaddressed.
This is a detector failure on a case that is in principle solvable by SL-G.

\medskip
\textbf{Repair:} retry=\xmark\enspace SL-G=\cmark\enspace DL=\xmark\enspace temp=\xmark\enspace temp\_loc=\xmark
}
\end{tcolorbox}

%% -----------------------------------------------------------------------
%  Example 3 — Distributed Deformation
%% -----------------------------------------------------------------------
\begin{tcolorbox}[breakable, width=\columnwidth,
  
  title={%
    \textbf{Ex.\,3:\ Distributed deformation — no intervention succeeds}
    \hfill{\small\texttt{sft-0.6B}, GPQA \texttt{gpqa\_recPzW1WqRnPs57D6}, $k=1$}},
  colback=red!3, colframe=red!40!black,
  fonttitle=\small\bfseries, before skip=6pt, after skip=4pt,
  left=4pt, right=4pt, top=3pt, bottom=3pt]
{\small
\textbf{Task (GPQA Diamond).}
Spin-$\tfrac{1}{2}$ particle with $\mu=\gamma S_z$, initially aligned with $\mathbf{B}$ along $+Z$.
Field switched to $+Y$ (same magnitude). What is the oscillation frequency of $\langle S_z\rangle$?

\medskip
\textbf{Failed rollout.} Model begins Larmor precession reasoning then stalls mid-sentence.

\medskip
\textbf{Interpretation.}
There is no dominant spike: the deformation is \emph{distributed}
($\Delta_{\mathrm{frac+}}{=}0.485$), meaning the specialist is demonstrably worse than the
ancestor at nearly \emph{half} of all token positions.
Coverage loss ($G_{\mathrm{cov,frac+}}{=}0.725$) compounds this — the ancestor spans
probability mass the specialist has lost at 72\% of steps, a pervasive structural gap.
No single injection can correct a tilt this broad; temperature resampling cannot either,
since every individual step is slightly wrong.
This is a case of \emph{Distributed Deformation}: the forgetting is not localized and
current interventions have no leverage point.

\medskip
\textbf{Repair:} retry=\xmark\enspace SL-G=\xmark\enspace DL=\xmark\enspace temp=\xmark\enspace temp\_loc=\xmark
}
\end{tcolorbox}

%% -----------------------------------------------------------------------
%  Example 4 — Early spike, high output variance, DL wins
%% -----------------------------------------------------------------------
\begin{tcolorbox}[breakable, width=\columnwidth,
  
  title={%
    \textbf{Ex.\,4:\ Early spike, high output variance — DL wins over SL-G}
    \hfill{\small\texttt{sft-1.7B}, CruxEval \texttt{sample\_577}, $k=1$}},
  colback=purple!3, colframe=purple!40!black,
  fonttitle=\small\bfseries, before skip=6pt, after skip=4pt,
  left=4pt, right=4pt, top=3pt, bottom=3pt]
{\small
\textbf{Task.}  Predict the output of a dict-aliasing function with \texttt{popitem}.\\
\textbf{Call:} \texttt{f([(1,\,'pos')])} \quad \textbf{Expected:} \texttt{[\{\}]}

\medskip
\textbf{Failed rollout.}  Model traces the first loop iteration correctly then cuts off:
\begin{quote}\ttfamily\footnotesize
d.popitem() removes the last item (since \texttt{dict} is a dictionary,
\texttt{popitem()} removes\ldots
\end{quote}

\medskip
\textbf{Junction spike:} token \textbf{36 / 1022} (\textbf{4\%} through the trace) —
at the initial problem-setup step, before any reasoning begins.

\medskip
\textbf{Interpretation.}
The spike is \emph{early} and the deformation is punctate ($\Delta_{\mathrm{frac+}}{=}0.067$),
but the output distribution at the spike is broad: many tokens compete at that position,
so flipping a single rank (SL-G) is insufficient to re-frame the problem.
Full probability-mass injection (DL) or elevated temperature overcomes the spread,
diversifying the initial trajectory enough to find the correct path.
The distinction from Ex.\,1 is the \emph{width} of the spike's output distribution —
not its position — which determines whether a rank-flip or a full prob-injection is needed.

\medskip
\textbf{Repair:} retry=\xmark\enspace SL-G=\xmark\enspace DL=\cmark\enspace temp=\cmark\enspace temp\_loc=\cmark
}
\end{tcolorbox}
