# Supplementary material for: Failed Reasoning Traces Tell You What Is Fixable (But Not by Reading Them)
Source: arXiv:2606.05145 source file (2026-06-03)
Supplement: Supplementary file 2 [file emnlp_appendix_endpoint_unique.tex]

% AUTO-GENERATED by paper-writing/render_tables.py — do not edit by hand
\begin{table}[htbp]
\centering
\small
\resizebox{\columnwidth}{!}{%
\begin{tabular}{llrrrr}
\toprule
Model & Task & Restoration & Endpoint-unique & \%~unique \\
\midrule
\modelA & CruxEval & 76 & 9 & \textbf{10.6\%} \\
\modelB & CruxEval & 128 & 17 & \textbf{11.7\%} \\
\modelC & CruxEval & 82 & 1 & 1.2\% \\
\midrule
\modelA & GPQA & 31 & 11 & \textbf{26.2\%} \\
\modelB & GPQA & 42 & 9 & \textbf{17.6\%} \\
\modelC & GPQA & 54 & 5 & 8.5\% \\
\midrule
SL-G & All & 312 & 34 & 9.8\% \\
DL & All & 251 & 33 & 11.6\% \\
\textbf{Any mixing} & All & 413 & 52 & \textbf{11.2\%} \\
\bottomrule
\end{tabular}%
}
\caption{\textbf{Endpoint-unique rescues (SL-G $\cup$ DL, $K{=}10$).}
For each specialist model and task, we classify all mixing rescues into
\emph{restoration-supported} (ancestor also passes at $K{=}10$) and
\emph{endpoint-unique} (neither specialist nor ancestor passes at $K{=}10$,
but the mixed distribution does). All endpoints evaluated under the same
$K{=}10$ sampling budget. grpo1p7b excluded (ancestor rollouts unavailable).}
\label{tab:endpoint-unique}
\end{table}
